# Supplementary material for: FactCHD: Benchmarking Fact-Conflicting Hallucination Detection
Source: arXiv:2310.12086 source file (2024-05-26)
Supplement: Supplementary file 1 [file appendix_case.tex]

\begin{table*}[ht!]
    \centering
    \resizebox{1.0\linewidth}{!}{
    \begin{tabularx}{1.2\linewidth}{bmb}
         \toprule[1.5pt] \textbf{ User Query} 
          & \textbf{Golden Label}
         & \textbf{Prediction} \\ 
         \midrule[0.75pt]
         
         \small {\textsc{Query: } Could you tell me the name of the series that Rick Yune was on that got canceled on December 12?

         \textsc{Response:} Rick Yune was on a series that canceled on December 12.}
         & FACTUAL
         &\small \textcolor{green!40!white}{FACTUAL.} The answer that Rick Yune was on a series that got canceled on December 12 is correct. Rick Yune was a cast member of the television series The Blacklist, which was canceled on December 12, 2014. Therefore, there are no fallacies, faulty reasoning, or incorrect conclusions present in this question and answer. \\
         \midrule[0.75pt]
         \small {\textsc{Query: } Could you inform me of the budget for the movie Poseidon? 
          
         \textsc{Response:}Poseidon had a budget of \$160 million.}
         & NON-FACTUAL
         &\small \textcolor{red!80!white}{NON-FACTUAL.} The answer that Poseidon had a budget of \$160 million is incorrect. Poseidon had a *budget of \$150 million*, not \$160 million. Therefore, this is a false incorrect conclusion.\\
           \midrule[0.75pt]
         \small {\textsc{Query:} 
          Could you inform me of the budget for the movie Poseidon? 
          
          \textcolor{gold}{\textsc{Retrieved:}
            1. Poseidon (film) - 7 million worldwide on a budget of \$160 million……
            2. Poseidon (DC Comics) - Poseidon is the name of a DC Comics deity who is based on the Greek god of the same name……  }

         \textsc{Response:} Poseidon had a budget of \$160 million.}

         & FACTUAL
         &\small \textcolor{green!40!white}{FACTUAL.} he answer that Poseidon had a budget of \$160 million is correct. The film had a budget of *160 million* and was released in the United States on May 12, 2006. Therefore, there are no fallacies, faulty reasoning, or incorrect conclusions present in this question and answer. \\
    \bottomrule[1.5pt]
    \end{tabularx}
    }
    \caption{Case example from the results of Alpaca-7B-LoRa (Tuning) and the illustration of the impact of retrieval enhancement.}
    \label{tab:case}
\end{table*}
