# Supplementary material for: FactCHD: Benchmarking Fact-Conflicting Hallucination Detection
Source: arXiv:2310.12086 source file (2024-05-26)
Supplement: Supplementary file 2 [file appendix_sample.tex]

\begin{table*}[!]
    \centering
    \resizebox{1.0\linewidth}{!}{
    \begin{tabularx}{1.2\linewidth}{mXm}
         \toprule[1.5pt] \textbf{\textsc{Query-Response}} 
          & \textbf{Factuality Pattern}
         & \textbf{Golden Label} \\ 
         \midrule[0.75pt]
         \small {\textsc{Query:} Could you provide me with the time frame during which Mount Rushmore was made? 
         
         \textsc{Response:} Mount Rushmore was made from 1927-1956. }
         & \textsc{Conventional}
         &\small \textcolor{red!80!white}{NON-FACTUAL.} The answer that Mount Rushmore was made from 1927-1956 is incorrect. The project's execution was overseen by Gutzon Borglum from 1927-1941, but construction was forced to end in late October 1941 due to lack of funding. Therefore, the time frame during which Mount Rushmore was made is from *1927-1941*, not 1956. This is a false conclusion.
\\
         \midrule[0.75pt]
         \small {\textsc{Query:}Which television series has the highest number of episodes among Beverly Hills, 90210, Salem, Around the World in 80 Days, Love of Life, and The Little Mermaid?


          
         \textsc{Response:}Among the given television series, Beverly Hills, 90210 has the highest number of episodes, with 293 episodes. Salem has 36 episodes, Around the World in 80 Days has 6 episodes, Love of Life has 7316 episodes, and The Little Mermaid has 31 episodes. Therefore, *Beverly Hills, 90210* has the highest number of episodes among all the given television series.
 }
         & \textsc{Comparison}
         &\small \textcolor{red!80!white}{NON-FACTUAL.} The answer that Beverly Hills, 90210 has the highest number of episodes among all the given television series is incorrect. While it is true that Beverly Hills, 90210 has 293 episodes, Love of Life actually has 7316 episodes, making it the television series with the highest number of episodes among the given options. Therefore, the answer contains faulty reasoning and incorrect conclusions.
 \\
           \midrule[0.75pt]
         \small {\textsc{Query:} What was the total fertility rate of the country that had diplomatic relations with the country where the film "Rock of Ages" was released in 1999?

          
         \textsc{Response:} The country that had diplomatic relations with the country where the film "Rock of Ages" was released in 1999 is Australia, and the total fertility rate of Australia in 1999 was *1.755*.",
}
         & \textsc{Multi-hops}
         &\small \textcolor{green!40!white}{FACTUAL.} The answer that the country that had diplomatic relations with the country where the film "Rock of Ages" was released in 1999 is Australia, and the total fertility rate of Australia in 1999 was 1.755 is correct. "Rock of Ages" was released in Serbia, which had diplomatic relations with China. China, in turn, had diplomatic relations with Australia. The total fertility rate of Australia in 1999 was indeed *1.755*. Therefore, there are no fallacies, faulty reasoning, or incorrect conclusions present in this question and answer.
 \\
           \midrule[0.75pt]
         \small {\textsc{Query:} 
          Can you provide the names of films composed by Danny Elfman and set in New York?
          
         \textsc{Response:} The films that meet the given criteria are "Sleepy Hollow" and "Taking Woodstock".}
         & \textsc{Set-Operation}
         &\small \textcolor{green!40!white}{FACTUAL.} The answer that "Sleepy Hollow" and "Taking Woodstock" are films composed by Danny Elfman and set in New York is correct. Danny Elfman composed the music for both "Sleepy Hollow" and "Taking Woodstock" and both films are set in New York. Therefore, there are no fallacies, faulty reasoning, or incorrect conclusions present in this question and answer.\\
    \bottomrule[1.5pt]
    \end{tabularx}
    }
    \caption{Sampling examples from trainset of {\ours} over four factuality  patterns}
    \label{tab:sample}
\end{table*}
